# Supplementary material for: Modeling and presentation of vaccination coverage estimates using data from household surveys
Source: arXiv:2004.03127 ancillary file (2020-04-07)
Supplement: Supplementary file 1 [file SuppInfo.pdf]

Supplementary materials for
"Modeling and presentation of vaccination coverage estimates using data from household surveys"

Tracy Qi Dong[1], Jon Wakefield[1,2]

[1] Department of Biostatistics, University of Washington, Health Sciences Building, NE Pacific St, Seattle, WA 98195, USA

[2] Department of Statistics, University of Washington, Padelford Hall, NE Stevens Way, Seattle, WA 98195, USA

# 1 Additional exploratory analysis of the 2018 NDHS data

In the 2018 NDHS, a total of 1389 survey clusters were selected to provide results representative at the national level as well as the state level. During the household listing operation, about 11 clusters were dropped as they were found to be insecure or vacated due to high levels of insurgency. In addition, due to extreme security issues in Borno state, 11 local government areas (LGAs, which are administrative-2 areas) where about 39% of Borno households reside, were dropped from the survey. Clusters selected from the dropped LGAs were replaced with other clusters from the remaining 16 LGAs in Borno. Consequently, state-level estimates for Borno are not representative for the dropped LGAs. Due to the non-proportional allocation of the sample to the different states and the possible differences in response rates, each survey respondent is assigned a sampling weight to approximate the relative number of people he or she represents in the total population.

We let $i$, $c$ and $k$ index states, survey clusters and children respectively and let $y_{ick}$ be the 0-1 indicator of whether child $k$, sampled at cluster $c$ in state $i$, has received MCV1 at the time of interview. We obtain the design-based Horvitz-Thompson (HT) direct estimates [1] of the MCV1 coverage $\hat{p}_i$ for state $i$ using

$$\hat{p}_i^{\text{HT}} = \frac{\sum_{c=1}^{m_i} \sum_{k=1}^{n_{ic}} y_{ick} \times w_{ick}}{\sum_{c=1}^{m_i} \sum_{k=1}^{n_{ic}} w_{ick}},$$

where $m_i$ is the number of survey clusters in state $i$, $n_{ic}$ is the total number of children sampled at cluster $c$ in state $i$, and $w_{ick}$ is the survey weight assigned to child $k$ sampled at cluster $c$ in state $i$. The survey weights are the reciprocal of the sampling probabilities with a non-response adjustment.

The 90% confidence intervals (CIs) associated with the direct estimates can also be calculated using design-based variance estimators that acknowledge the stratification and clustering. All design-based estimation is implemented using the `survey` package [2] in the `R` computing environment [3].

Figure S1 shows the maps for the state-level HT direct coverage estimates $\hat{p}_i^{\text{HT}}$ and the widths of the associated 90% CIs. In general, the northern states of Nigeria have lower estimated MCV1 coverage than the southern states. Most 90% CI widths are relatively narrow, indicating moderate confidence in the state-level direct estimates.

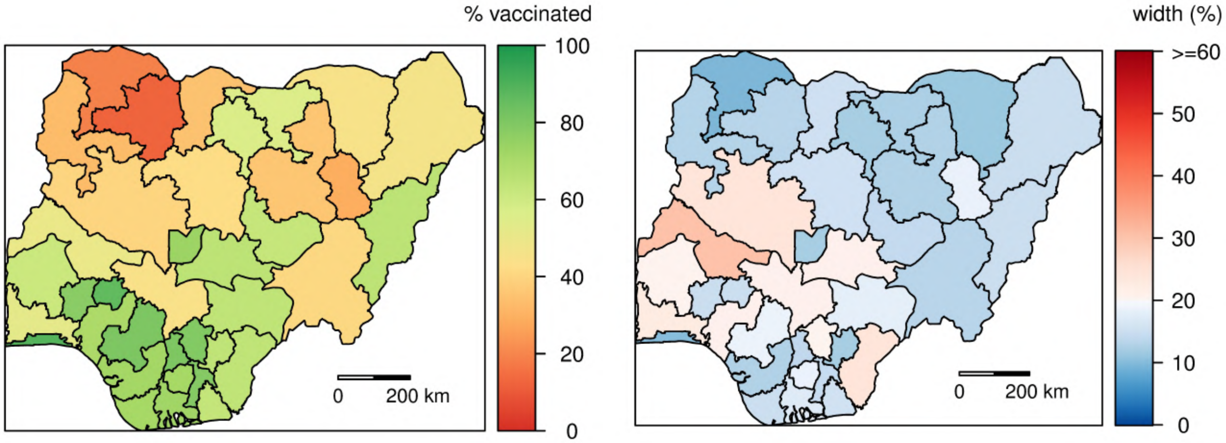


Figure S1: Left: state-level Horvitz-Thompson direct estimates of MCV1 coverage among children aged 12–23 months. Right: the widths of the associated 90% confidence intervals.

As mentioned in Section 2 of the main paper, the cluster-level observed coverage seem to show spatial correlation: clusters that are closer to each other tend to have similar observed coverage (Figure 1). However, it is not uncommon to see clusters in close proximity having significantly different observed coverage, which could be outcome variation explained by factors other than spatial location and/or sampling variation. Here, we take a closer look at the variation and spatial correlation in cluster-level observed coverage by examining the empirical semi-variogram [4] based on the following non-spatial binomial mixed model:

$$
\begin{aligned}
Y_{ic}|p_{ic} &\sim \text{Binomial}\left(n_{ic}, p_{ic}\right) \\
\text{logit}(p_{ic}) &= \alpha + \boldsymbol{\beta}^{\top}\boldsymbol{x}_{ic} + C_{ic} \\
C_{ic} &\sim_{iid} \text{Normal}\left(0, \sigma_C^2\right),
\end{aligned} \tag{1}
$$

where $\sim_{iid}$ is short for "are independently and identically distributed as". Here, $Y_{ic}$ is the random variable representing the number of vaccinated children out of $n_{ic}$ who are sampled in cluster $c$ of state $i$, $p_{ic}$ is the probability of vaccination parameter in the binomial model that represents the cluster-level vaccination coverage, and $\boldsymbol{x}_{ic}$ is the vector of covariates associated with cluster $c$ in state $i$. We use

the same covariates selected by Utazi *et al.* [5]. These covariates are: poverty, aridity, log-transformed night-time lights, log-transformed travel time and enhanced vegetation index (EVI). The details of how the covariates are processed for model fitting can be found in the next section.

The semi-variogram is a standard tool for examining spatial dependence. Figure S2 shows the empirical semi-variogram based on the posterior medians of the random effects $C_{ic}$, estimated using the integrated nested Laplace approximation (INLA) approach [6], implemented in the `INLA` package in `R`. The semi-variogram shows an increasing trend with increasing distance between points, that flattens out at a range of around 250 km, indicating that locations farther apart than that distance are not spatially correlated. In addition, the semi-variogram exhibits a considerable *nugget* effect when the spatial distance is very small. The *nugget* is typically associated with "measurement error" and small-scale variation [4]. This hints at the existence of non-spatial excess variation in the outcome at the cluster level, in addition to the variation explained by covariates and the spatial field.

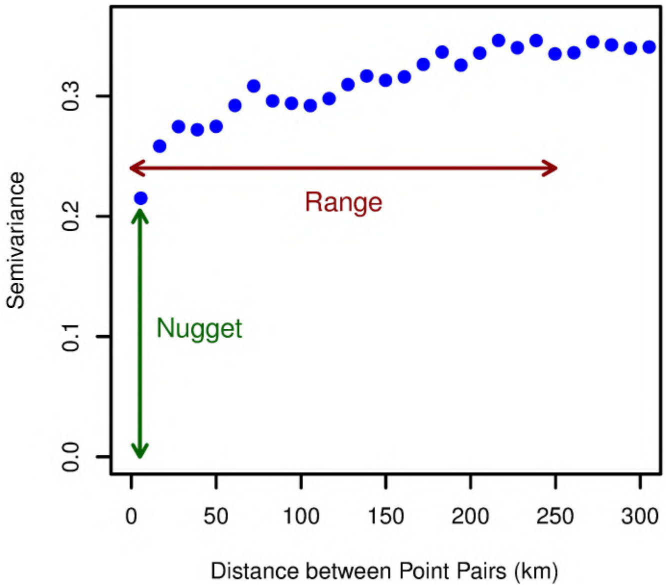


Figure S2: The empirical semi-variogram for MCV1 coverage in Nigeria based on the posterior medians of the random effects $C_{ic}$ in the non-spatial binomial mixed model (1).

## 2 Covariate data processing

Five geospatial covariates have been used in our analyses: poverty, aridity, log-transformed night-time lights, log-transformed travel time and enhanced vegetation index (EVI). These are the same covariates selected by Utazi *et al.* in their 2018 paper [5]. Below are the sources of the covariate data:

- Poverty: Worldpop 2010 estimates of proportion of people per grid square living in poverty, as defined by $2 a day threshold. URL: `https://www.worldpop.org/geodata/summary?id=1267`

- Aridity: Consortium for Spatial Information (CGIAR-CSI) 2018 Global Aridity Index map. URL: `http://www.cgiar-csi.org/data/global-aridity-and-pet-database`)
- Nighttime lights: NOAA VIIRS Nighttime Lights 2018 October data. (`https://www.ngdc.noaa.gov/eog/viirs/download_dnb_composites.html`).
- Travel time: Malaria Mapping Project 2015 Map of Travel Time to Cities. URL: `https://malariaatlas.org/explorer/`
- EVI: MOD13A3 MODIS/Terra vegetation Indices Monthly L3 Global 1km SIN Grid V006, 2018 October data. URL: `https://doi.org/10.5067/MODIS/MOD13A3.006`

We standardized each covariate surface into a gridded layer at a $1 \times 1$ km resolution using the `raster` package in `R`. To extract the covariate values at each DHS cluster location and account for the jittering, we overlay the cluster GPS coordinates with the covariate layers and create 2 km and 5 km buffers around clusters in urban and rural areas respectively. The mean values of the grid cells within the buffers were extracted to be used as the covariate values for the cluster-level survey data. This procedure is adopted from the methods used by Utazi *et al.* in their 2018 paper [5].

For pixel-level coverage estimation, we standardized the Worldpop UN adjusted population layer for 2018 (URL: `https://www.worldpop.org/geodata/summary?id=28029`) into a gridded population surface at $1 \times 1$ km resolution. We overlay the controids of the pixels with the standardized covariate layers and extract the corresponding covariate values without creating any buffer.

## 3 Urban/rural classification of pixels on the gridded population surface

In addition to extracting covariate values for each pixel on the prediction grid, we also need to classify each pixel into urban/rural to account for the survey stratification in our prediction. We take the following steps to carry out the classification:

1. Using Table A.1 in the 2018 DNHS report [7], we obtain the urban population proportion within each state.
2. For a given state, we rank the pixels on the gridded population surface **within the state** by descending population size. We start from the top of the ranked list and classify each pixel as urban until the total urban population proportion reach the DHS reported proportion for that state (from step 1). The rest of the pixels in the state will be classified as rural.
3. We repeat step 2 for each state in Nigeria.

This procedure essentially classify the more densely populated pixels within each state to be urban such that the urban population proportion within each state matches what was stated in the DHS report. We emphasize that this is an approximate procedure, since the result of our classification procedure will not

match the urban/rural areas in Nigeria exactly — our approach is carried out at the pixel level, whereas the urban/rural areas in Nigeria have been classified at the census enumeration area (EA) level.

# 4 The approximated enumeration area (EA) map

As discussed in Section 3 of the main paper, the complete sampling frame of EAs is almost always unavailable. Therefore, we need to create an approximated EA map for aggregating cluster-level estimates to form areal level (e.g., state- or LGA-level) coverage estimates. We take the following steps to create the approximated EA map:

1. Using Table A.2 in the 2018 DNHS report [7], we obtain the number of urban and rural EAs within each state.

2. We overlay the gridded population surface from Section 3 with the state/LGA boundaries and assign each pixel to a state/LGA based on its centroid location. We can then calculate the total urban and rural population within each state and within each LGA.

3. Within each state, we can calculate the state-level **average urban/rural EA size** by dividing the urban/rural population by the number of urban/rural EAs in the state.

4. Assuming all the LGAs within a state have the same average urban/rural EA population sizes as the state-level average urban/rural EA population sizes, we can calculate the number of urban/rural EAs within each LGA, denoted $C_j^{(u)}$ and $C_j^{(r)}$ for LGA $j$, by dividing the urban/rural population by the average urban/rural EA size.

5. Within the urban pixels in LGA $j$, we can create an approximated urban EA map by sampling $C_j^{(u)}$ pixels with probability proportional to population size with replacement. Pixels with large population counts might be sampled multiple times, meaning that there might be more than one EAs located in a pixel. We can do the same for the rural pixels and create an approximate rural EA map.

6. We repeat steps 3-5 for each state and LGA in Nigeria.

This procedure creates an approximate EA map that matches the summary EA information provided in the DHS report.

# 5 Lono-Binomial distribution

The Lono-Binomial distribution is the compound distribution where the $p$ parameter in the binomial distribution as being randomly drawn from a logit-normal distribution. We use this name to emphasize

the parallel between this distribution and the Beta-Binomial distribution. Specifically, a random variable $Y \sim$ Lono-Binomial $(n, \eta, \sigma_\delta^2)$ if

$$
\begin{aligned}
&Y|q \sim \text{Binomial}\,(n, q)\\
&\text{logit}\,(q)\,|\eta, \sigma_\delta^2 = \eta + \delta\\
&\delta \sim_{iid} \text{Normal}\left(0, \sigma_\delta^2\right).
\end{aligned}
$$

The parameter $\sigma_\delta^2 > 0$ characterizes the degree of overdispersion, with higher $\sigma_\delta^2$ value corresponding to more overdispersion. The limiting case of a Lono-Binomial distribution at $\sigma_\delta^2 = 0$ is a binomial distribution. The likelihood is given by

$$\Pr(Y|\eta, \sigma_\delta^2) = \int_q \Pr(Y|q) \times \pi(q|\eta, \sigma_\delta^2)\; dq.$$

This likelihood has no closed form but is overdispersed relative to the binomial. The marginal mean and variance are

$$
\begin{aligned}
\text{E}[Y] &\approx n \times \text{expit}\left(\frac{\eta}{\sqrt{1 + h^2\sigma_\delta^2}}\right)\\
\text{var}(Y) &= \text{E}_\delta[\text{var}(Y|\delta)] + \text{var}_\delta(\text{E}[Y|\delta])
\end{aligned}
$$

where $h = \frac{16\sqrt(3)}{15\pi}$.

# 6 Model fitting and assessment details

All models were fitted using the INLA approach [6] implemented in the `INLA` package in `R`. For the intercept $\alpha$, a N(0, 0) prior is used, where the format is N(mean,precision); this prior is improper but the intercept is well estimated. For the other fixed effect parameters (i.e., $\boldsymbol{\beta}, \gamma$) We used N(0, 0.001) priors. We used the Penalized Complexity (PC) priors [8] for the hyperparameters of the random effects — these are typically the most sensitive to the prior choice. For the spatial range $\rho$, we set a PC prior so that the median effective range is at a fifth of the diameter of the spatial domain. For the variance hyperparameters, we set PC priors so that $\Pr(\sigma_\epsilon > 1) = \Pr(\sigma_S > 1) = \Pr(\sigma_\delta > 1) = 0.01$.

For model validation, we used the hold-out method of cross-validation, setting aside data from an entire state each time. Within a hold-out state, let $y_c$ and $n_c$ be the number of vaccinated and sampled children at cluster $c$, and $\hat{p}_c = \frac{y}{n}$ be the observed coverage at cluster $c$. In addition, let $\tilde{p}_c$ be the posterior median of the coverage estimate at cluster $c$ obtained from fitting the model on data from other states. Using the hold-out data from $m$ cluster locations, we computed the following model evaluation criteria:

- Bias $= \frac{1}{m}\sum_c(\tilde{p}_c - \hat{p}_c)$.

- Mean Absolute Error (MAE) $= \frac{1}{m}\sum_c |\tilde{p}_c - \hat{p}_c|$.
- Root Mean Square Error (RMSE) $= \sqrt{\frac{1}{m}\sum_c (\tilde{p}_c - \hat{p}_c)^2}$.

Table S1 shows the posterior medians and 2.5% and 97.5% quantiles of the regression coefficients for covariates. Figures S3-S5 show the maps of the posterior medians (top row) and the widths of 90% credible intervals (botton row) for the estimated MCV1 coverage at the $1 \times 1$ km pixel (left), LGA (middle) and state (right) levels, based on the *Binomial NN*, *Beta-Binomial OD* and *Binomial TS* model that include the urban/rural strata variable. Note that the *Lono-Binomial OD* model and the *Binomial TS* model have the same estimates for all model parameters. However, their prediction surfaces are different (Figure 2 in the main paper v.s. Figure S5 in this document), because the two models have different targets of inference (see equations (8) and (9) in the main paper).

| Model Class | Strata Included? | Intercept | Aridity | Poverty | EVI | Travel Time | Night Light |
|---|---|---|---|---|---|---|---|
| Binomial NN | No Strata | 1.7<br>(0.21, 3.3) | 0.57<br>(0.13, 1.0) | -2.2<br>(-4.0, -0.39) | -0.0085<br>(-0.13, 0.11) | -0.093<br>(-0.19, 0.0012) | 0.31<br>(0.14, 0.50) |
| | Strata | 1.5<br>(-0.065, 3.0) | 0.53<br>(0.08, 0.97) | -2.2<br>(-4.1, -0.45) | 0.0048<br>(-0.12, 0.13) | -0.046<br>(-0.15, 0.053) | 0.25<br>(0.071, 0.43) |
| Beta-Binomial OD | No Strata | 2.1<br>(0.6, 3.7) | 0.26<br>(-0.36, 0.83) | -2.4<br>(-4.2, -0.75) | -0.044<br>(-0.16, 0.074) | -0.067<br>(-0.15, 0.021) | 0.26<br>(0.09, 0.44) |
| | Strata | 1.9<br>(0.33, 3.5) | 0.21<br>(-0.42, 0.78) | -2.5<br>(-4.3, -0.8) | -0.027<br>(-0.15, 0.09) | -0.023<br>(-0.12, 0.068) | 0.21<br>(0.029, 0.39) |
| Lono-Binomial OD | No Strata | 2.1<br>(0.50, 3.8) | 0.29<br>(-0.40, 0.90) | -2.8<br>(-4.7, -1.0) | -0.046<br>(-0.17, 0.081) | -0.068<br>(-0.16, 0.025) | 0.30<br>(0.12, 0.49) |
| | Strata | 2.1<br>(0.50, 3.8) | 0.23<br>(-0.47, 0.84) | -2.9<br>(-4.8, -1.1) | -0.028<br>(-0.16, 0.099) | -0.018<br>(-0.12, 0.08) | 0.23<br>(0.044, 0.42) |
| Binomial TS | No Strata | 2.1<br>(0.50, 3.8) | 0.29<br>(-0.40, 0.90) | -2.8<br>(-4.7, -1.0) | -0.046<br>(-0.17, 0.081) | -0.068<br>(-0.16, 0.025) | 0.30<br>(0.12, 0.49) |
| | Strata | 2.1<br>(0.50, 3.8) | 0.23<br>(-0.47, 0.84) | -2.9<br>(-4.8, -1.1) | -0.028<br>(-0.16, 0.099) | -0.018<br>(-0.12, 0.08) | 0.23<br>(0.044, 0.42) |

Table S1: Estimates of parameters for each model. Reported are the posterior medians and 2.5% and 97.5% quantiles of the regression coefficients for covariates. Note that the estimates for the coefficients of covariates are not directly comparable because the covariates are measured on different scales.

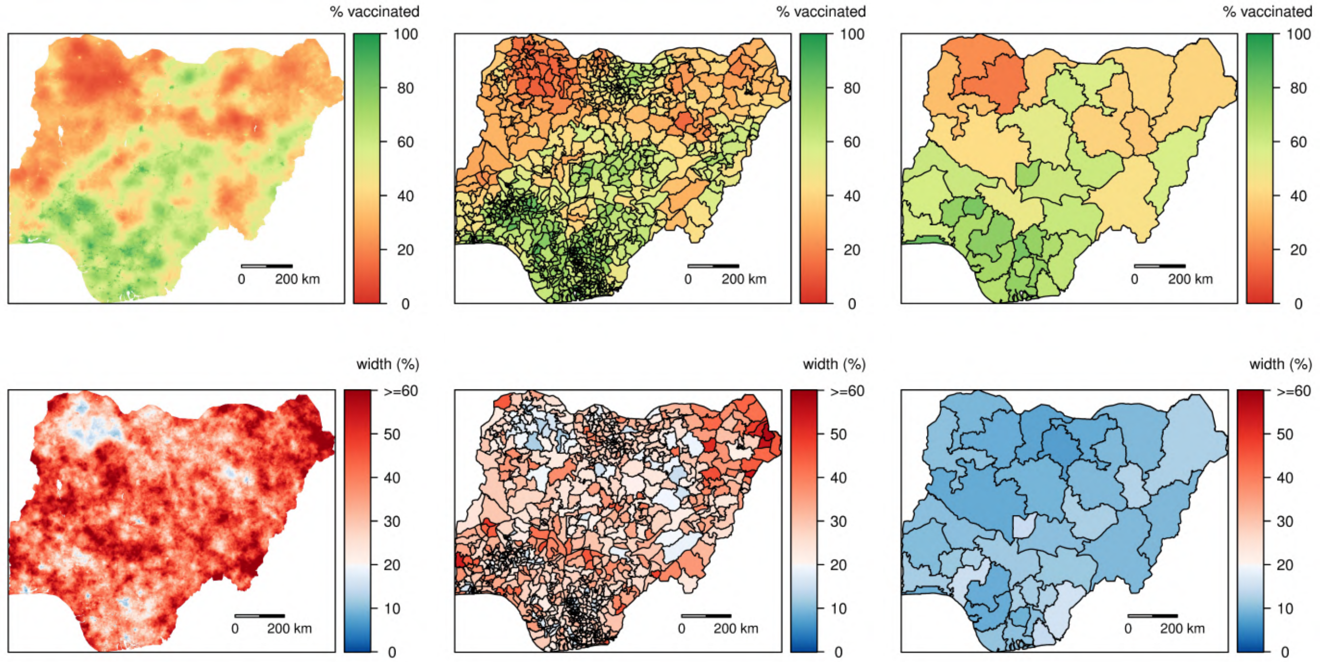


Figure S3: Maps of the posterior medians (top row) and the widths of 90% credible intervals (botton row) for the estimated MCV1 coverage at the $1 \times 1$ km pixel (left), LGA (middle) and state (right) levels, based on the *Binomial NN* model that includes the urban/rural strata variable.

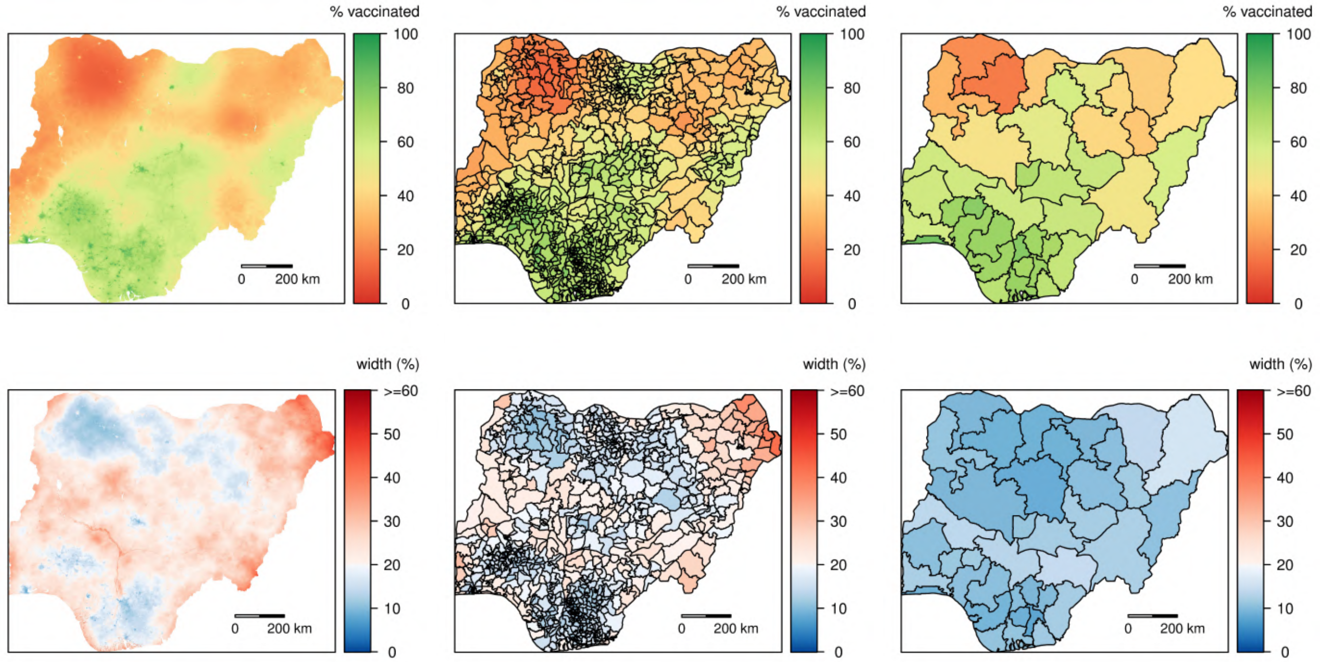


Figure S4: Maps of the posterior medians (top row) and the widths of 90% credible intervals (botton row) for the estimated MCV1 coverage at the $1 \times 1$ km pixel (left), LGA (middle) and state (right) levels, based on the *Beta-Binomial OD* model that includes the urban/rural strata variable.

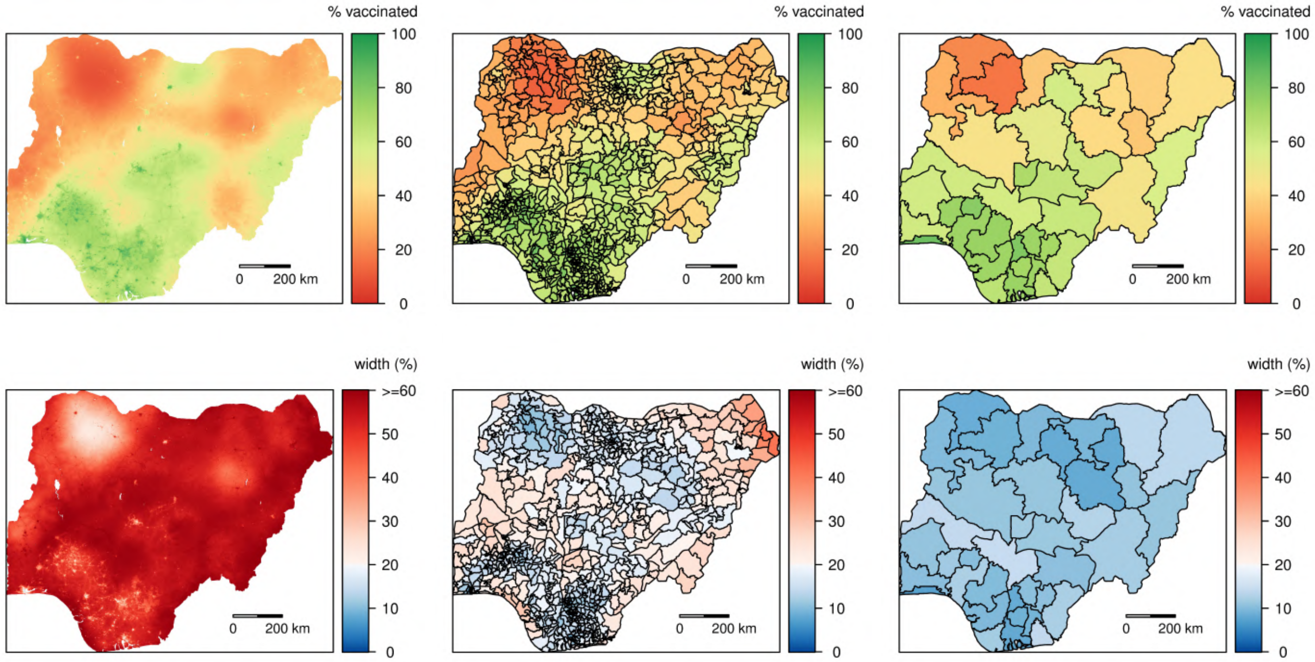


Figure S5: Maps of the posterior medians (top row) and the widths of 90% credible intervals (botton row) for the estimated MCV1 coverage at the $1 \times 1$ km pixel (left), LGA (middle) and state (right) levels, based on the *Binomial TS* model that includes the urban/rural strata variable.

## 7 Coefficient of variation (CV) as an uncertainty measure

Consider the vaccination coverage $p$ for a generic area. Let $\theta = \frac{p}{1-p}$ be the odds, and $\phi = \log(\theta) = \text{logit}(p)$ be the log odds. We assume that the posterior for the log odds $\phi$ in a generic area approximately follows a Normal$(\hat{\phi}, \hat{\sigma}^2)$ distribution, where $\hat{\phi}$ and $\hat{\sigma}^2$ are posterior estimates of $\mathsf{E}[\phi|\boldsymbol{y}]$ and var$(\phi|\boldsymbol{y})$. This is equivalent to the posterior for the odds $\theta$ following a LogNormal$(\hat{\phi}, \hat{\sigma}^2)$ distribution, with mean, variance and coefficient of variation (CV)

$$\begin{aligned}
\mathsf{E}\left[\theta|\boldsymbol{y}\right] &= \exp\left(\hat{\phi} + \frac{\hat{\sigma}^2}{2}\right), \\
\text{var}\left(\theta|\boldsymbol{y}\right) &= \mathsf{E}\left[\theta|\boldsymbol{y}\right]^2 \times \left(\exp(\hat{\sigma}^2) - 1\right), \\
\text{CV}\left(\theta|\boldsymbol{y}\right) &= \frac{\sqrt{\text{var}\left(\theta|\boldsymbol{y}\right)}}{\mathsf{E}\left[\theta|\boldsymbol{y}\right]} = \sqrt{\exp(\hat{\sigma}^2) - 1} \approx \sqrt{\hat{\sigma}^2} = \hat{\sigma},
\end{aligned}$$

i.e., the posterior standard deviation sd$(\phi|\boldsymbol{y})$.

Now we consider the 100(1 - $\alpha$)% posterior credible interval (CI) for $\theta$. The ratio of the higher bound to the lower bound of the CI is

$$\frac{\text{CI}_{\text{hi}}\left(\theta|\boldsymbol{y}\right)}{\text{CI}_{\text{lo}}\left(\theta|\boldsymbol{y}\right)} = \frac{\exp\left(\hat{\phi} + z_{\alpha/2}\hat{\sigma}\right)}{\exp\left(\hat{\phi} - z_{\alpha/2}\hat{\sigma}\right)} = \exp\left(2z_{\alpha/2}\hat{\sigma}\right) \approx \exp\left(2z_{\alpha/2}\text{CV}\left(\theta|\boldsymbol{y}\right)\right),$$

where $z_{\alpha/2}$ is the $\alpha/2$ quantile of a standard normal random variable. Hence,

$$\text{CV}\left(\theta|\boldsymbol{y}\right) \approx \frac{1}{2z_{\alpha/2}} \log\left(\frac{\text{CI}_{\text{hi}}\left(\theta|\boldsymbol{y}\right)}{\text{CI}_{\text{lo}}\left(\theta|\boldsymbol{y}\right)}\right),$$

so that there is a direct relationship between the posterior CV and the ratio of higher end to lower end of the posterior credible interval.

This justifies using hatching based on the posterior CVs of area-level vaccination coverage odds. For example, Figure S6 shows a map of the posterior medians of the MCV1 coverage estimates for Nigeria 37 states, with hatching density proportional to the posterior CV of the vaccination odds. The results are based on 1000 posterior samples of the MCV1 coverage estimates from the *Lono-Binomial OD* model that includes the urban/rural strata variable.

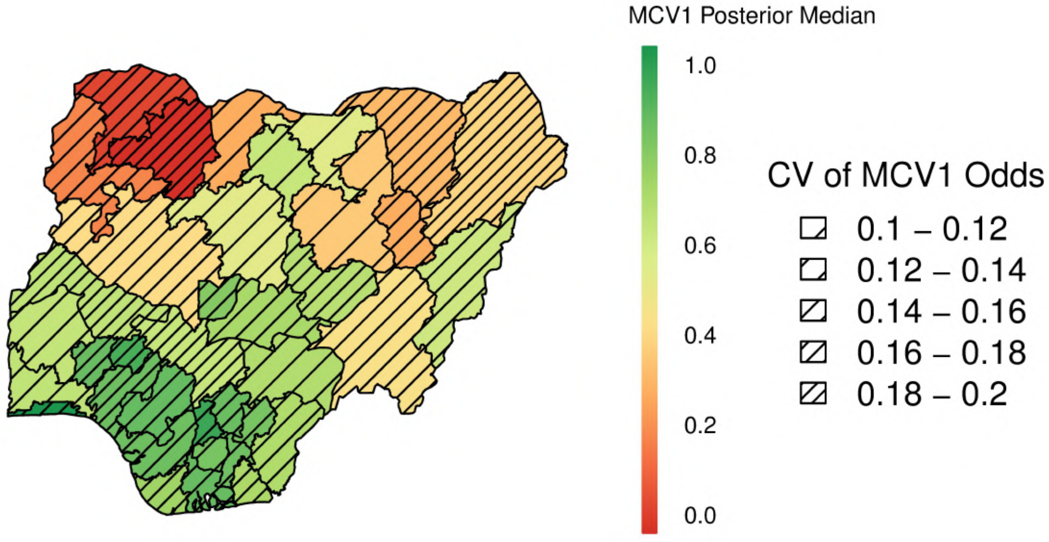


Figure S6: Map of the posterior medians of the MCV1 coverage estimates for Nigeria's 37 states, with hatching density proportional to the posterior coefficient of variation (CV) of the vaccination odds. The results are based on 1000 posterior samples of the MCV1 coverage estimates from the *Lono-Binomial OD* model that includes the urban/rural strata variable.

# 8 Additional plots for the posterior ranking distributions

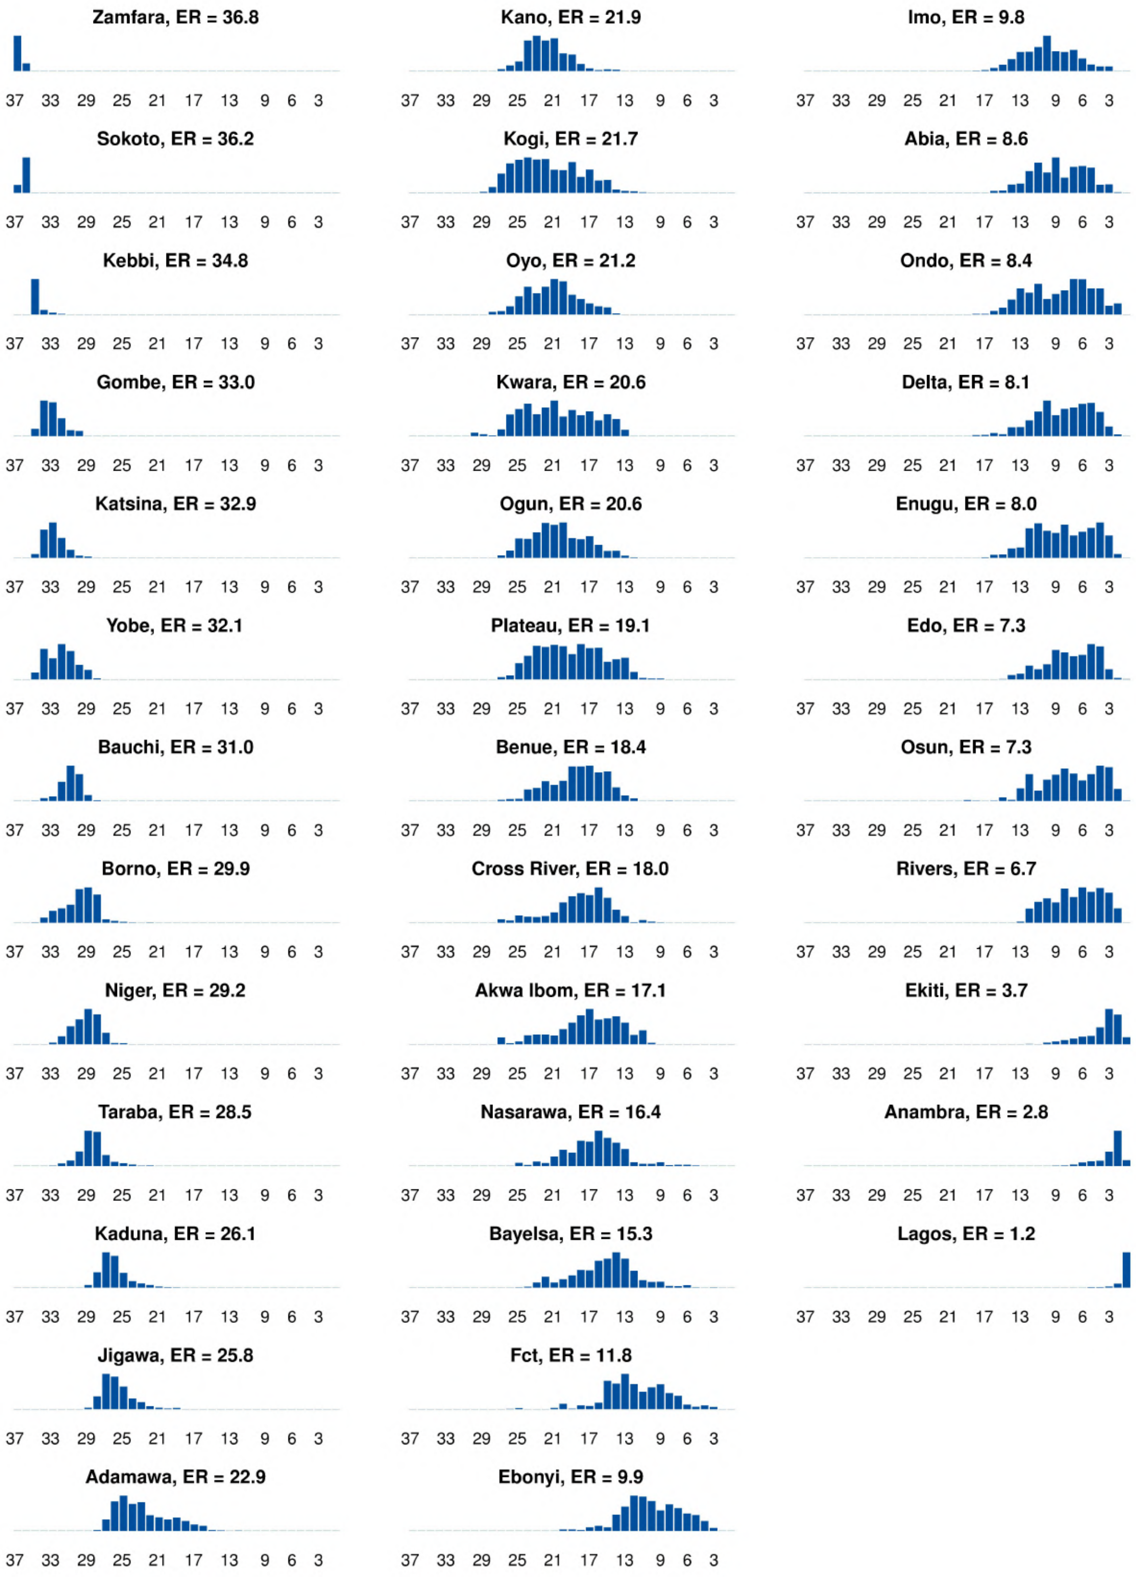


Figure S7: Posterior ranking distributions of all 37 states in Nigeria with their expected ranks (ER) based on 1000 posterior samples of the MCV1 coverage estimates from the *Lono-Binomial OD* model that includes the urban/rural strata variable.

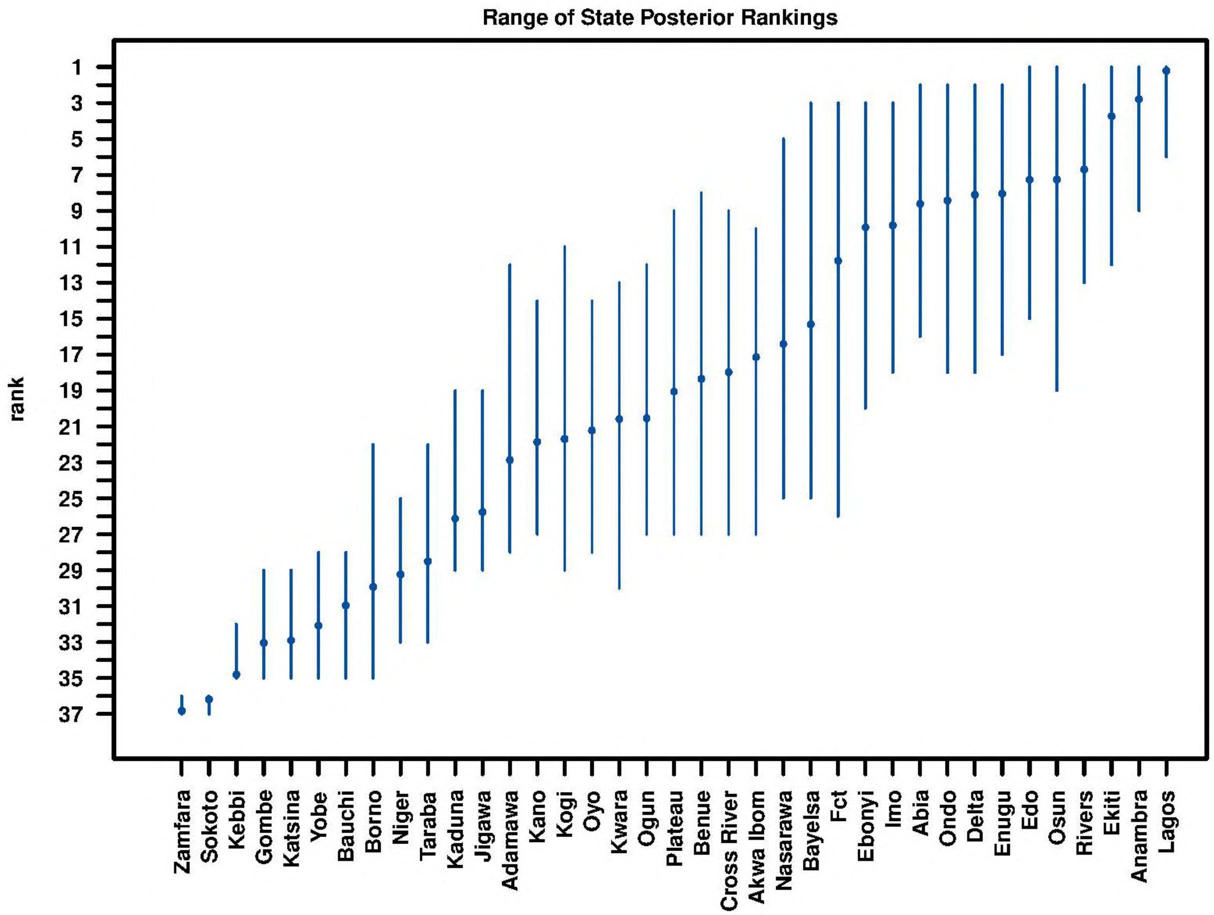


Figure S8: The range of the posterior rankings of all 37 states in Nigeria with their expected ranks (ERs) based on 1000 posterior samples of the MCV1 coverage estimates from the *Lono-Binomial OD* model that includes the urban/rural strata variable. The points indicate the ERs of the states, and the vertical line segments mark the complete range of the posterior rankings of the states.

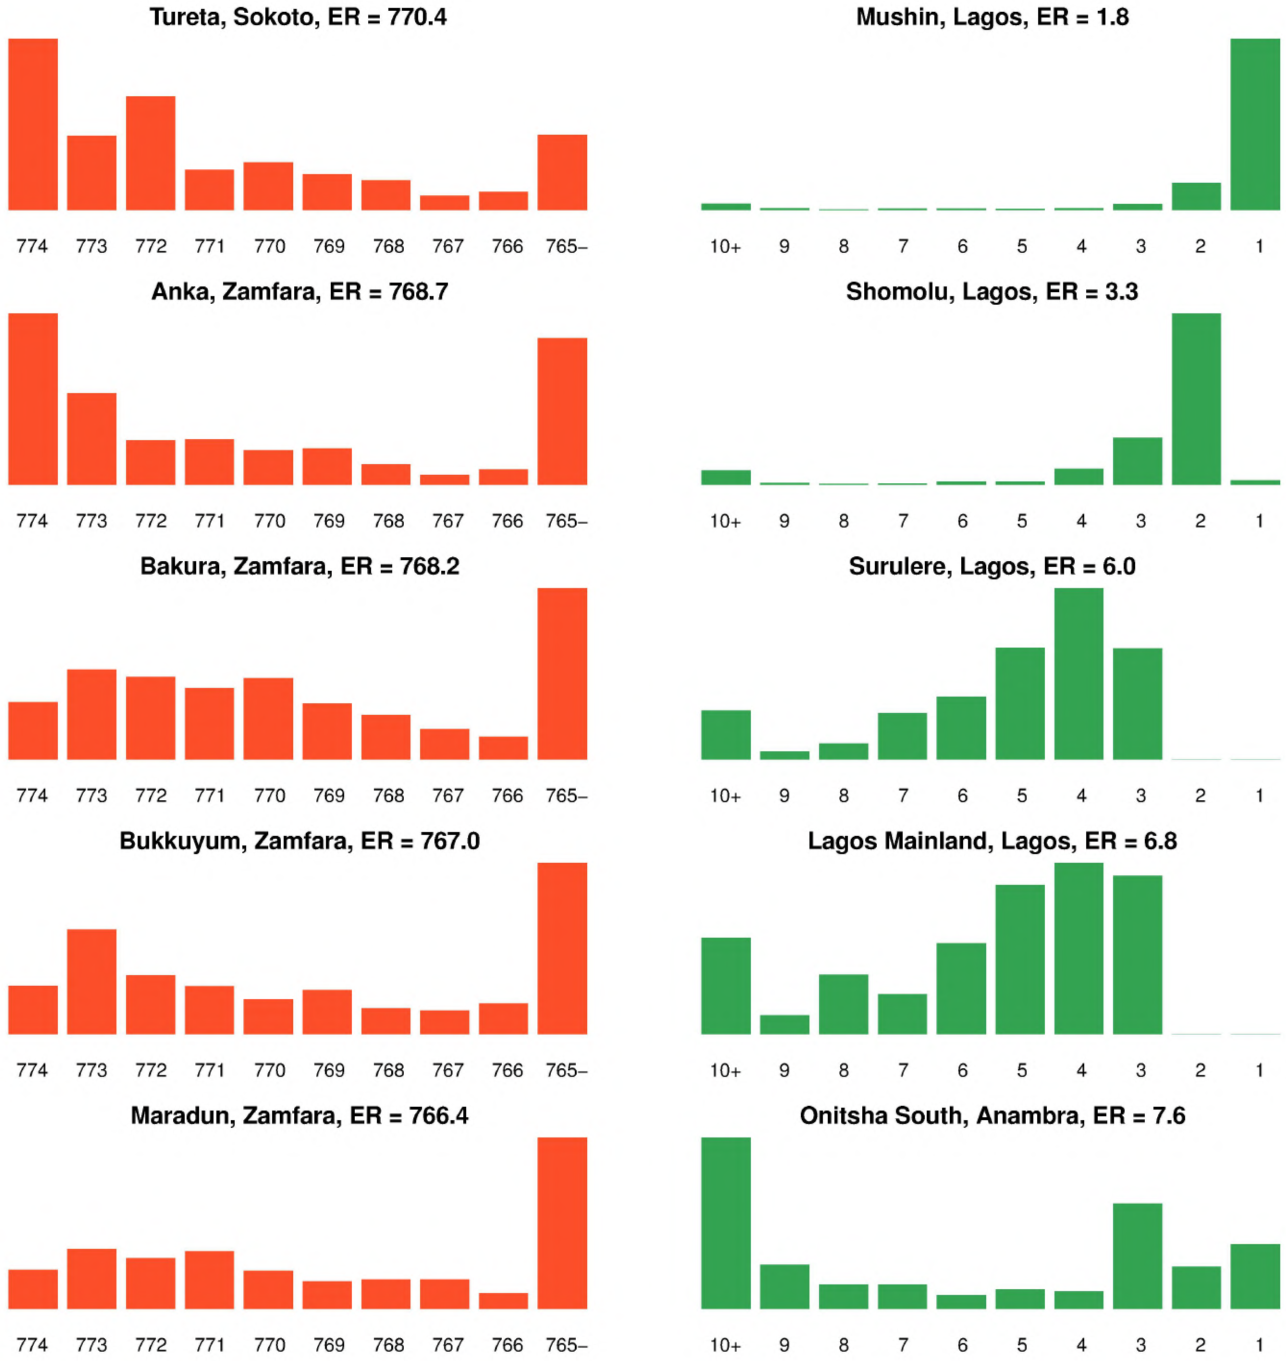


Figure S9: Posterior ranking distributions of the 5 LGAs with the lowest (left column) and 5 with the highest (right column) expected ranks (ERs) based on 1000 posterior samples of the MCV1 coverage estimates of Nigeria's 774 LGAs from the *Lono-Binomial OD* model that includes the urban/rural strata variable.

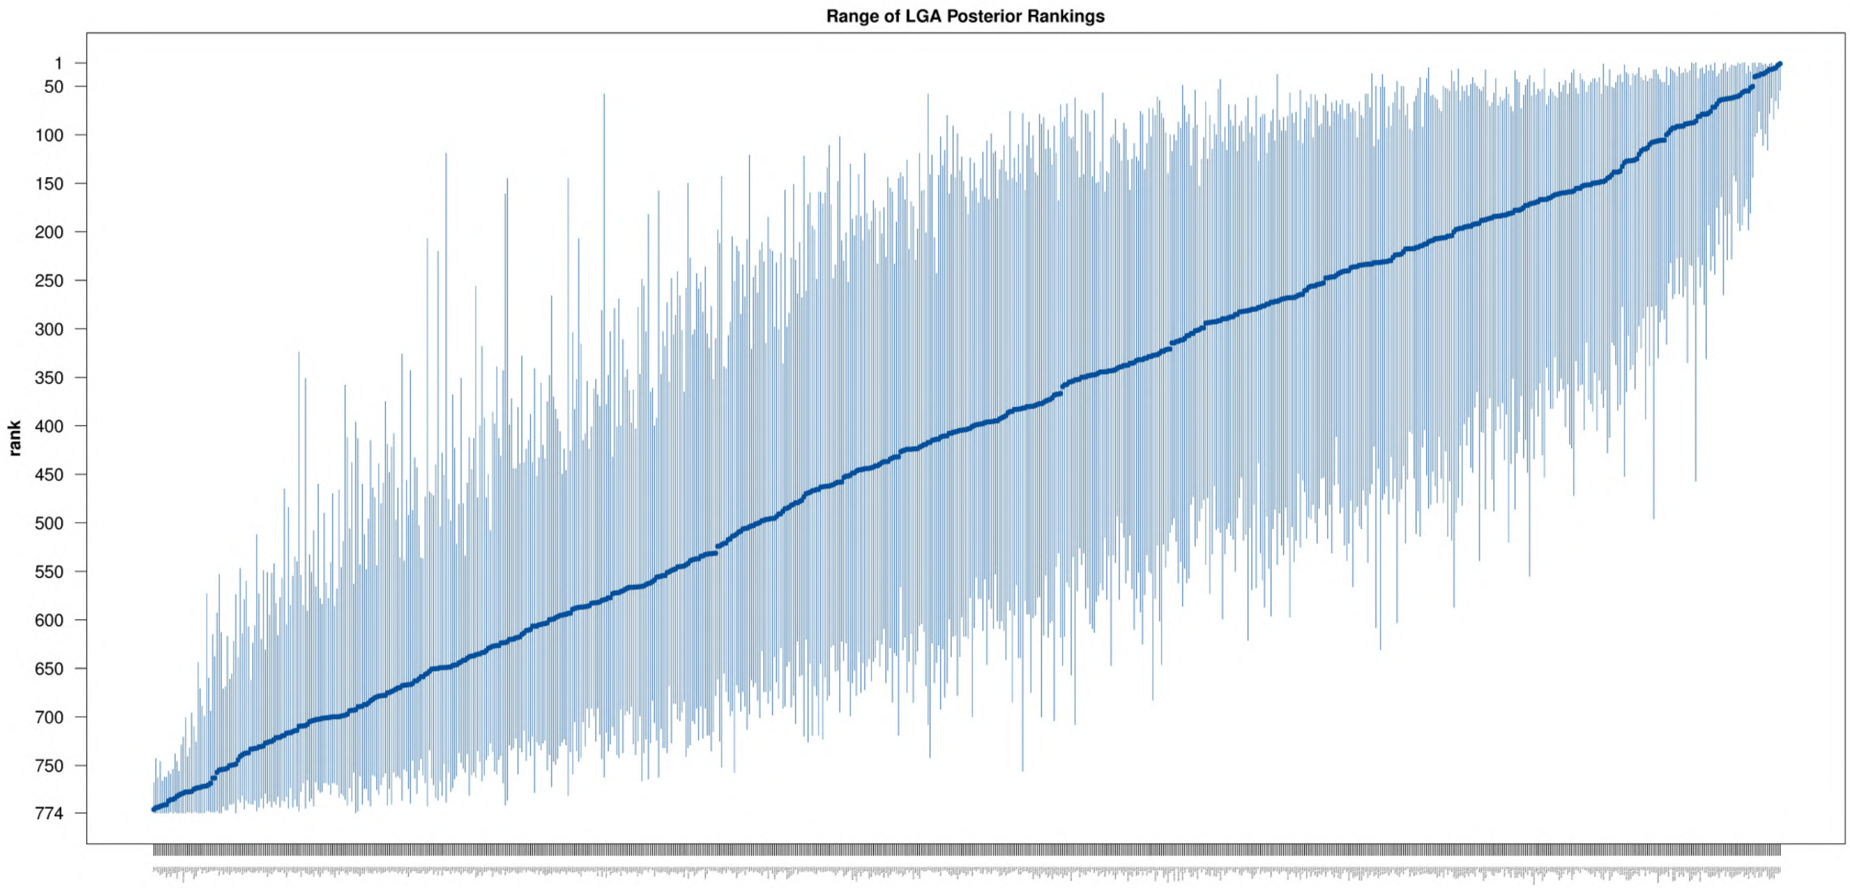


Figure S10: The range of the posterior rankings of all 774 LGAs in Nigeria with their expected ranks (ER) based on 1000 posterior samples of the MCV1 coverage estimates from the *Lono-Binomial OD* model that includes the urban/rural strata variable. The points indicate the expected ranks (ER) of the LGAs, and the vertical line segments mark the complete range of the posterior rankings of the LGAs.

# 9 Additional plots for the true classification probability (TCP) and average ture classification probability (ATCP)

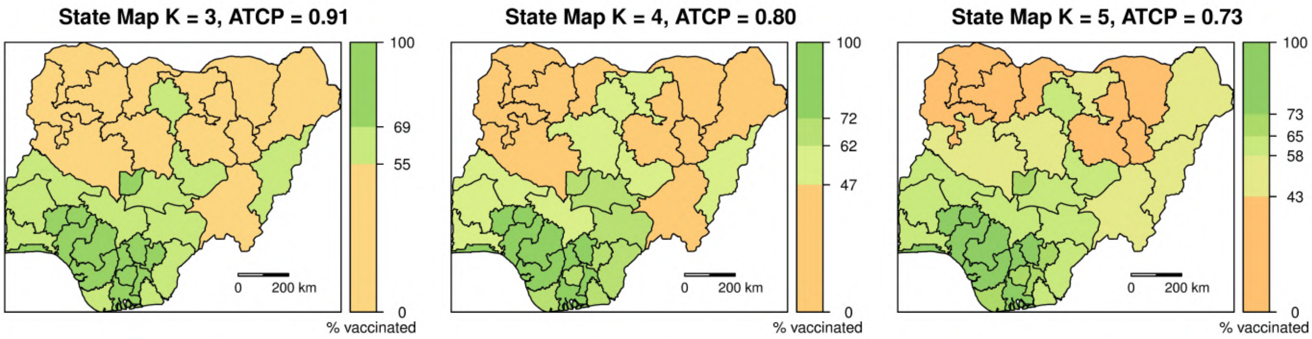


Figure S11: Maps of MCV1 coverage estimates at the state level using discrete color scales with $K = 3, 4$ and $5$ quantile intervals. For each $K$ , the color scale is formed by creating the intervals $[L_0, L_1), \ldots, [L_{K-1}, L_K]$, where $L_0 = 0\%$, $L_K = 100\%$, and $L_k$ equals the $100 \times k/K$ quantile of the pooled posterior samples of the state-level coverage estimates based on the *Lono-Binomial OD* model that includes the urban/rural strata variable.

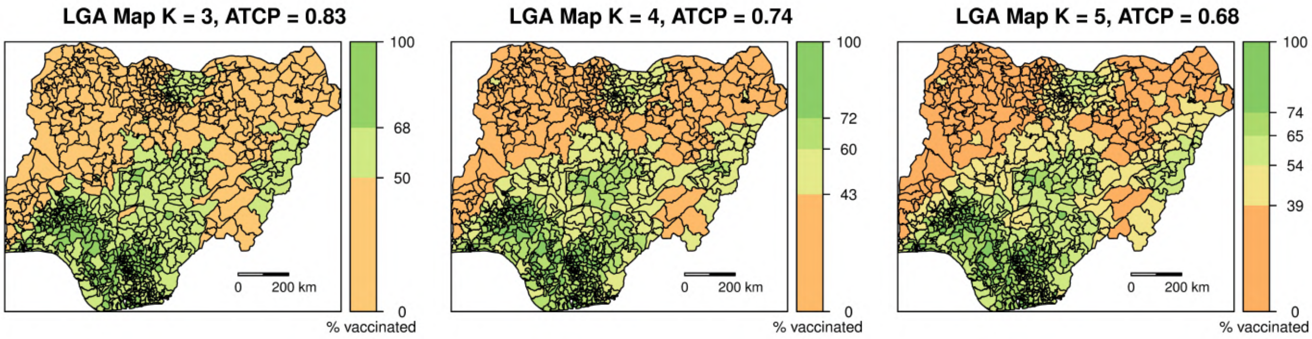


Figure S12: Maps of MCV1 coverage estimates at the LGA level using discrete color scales with $K = 3, 4$ and $5$ quantile intervals. For each $K$ , the color scale is formed by creating the intervals $[L_0, L_1), \ldots, [L_{K-1}, L_K]$, where $L_0 = 0\%$, $L_K = 100\%$, and $L_k$ equals the $100 \times k/K$ quantile of the pooled posterior samples of the LGA-level coverage estimates based on the *Lono-Binomial OD* model that includes the urban/rural strata variable.

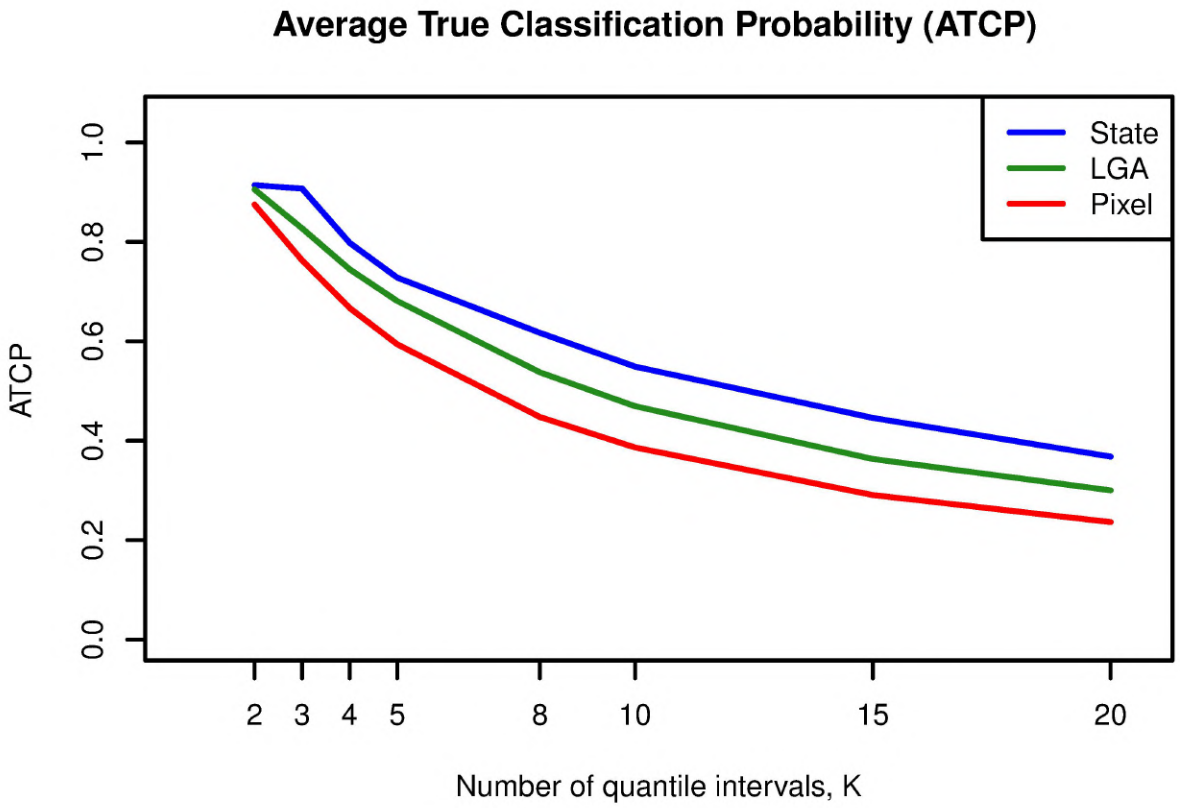


Figure S13: The average ture classification probabilities (ATCP) corresponding to the state, LGA and $1 \times 1$ km pixel maps with discrete color scales defined by various number of quantile intervals $K$. For each $K$ within each spatial resolution (state, LGA or pixel), the quantile intervals are formed by creating the intervals $[L_0, L_1), \ldots, [L_{K-1}, L_K]$, where $L_0 = 0\%$, $L_K = 100\%$, and $L_k$ equals the $100 \times k/K$ quantile of the pooled posterior samples of the coverage estimates at that spatial scale based on the *Lono-Binomial OD* model that includes the urban/rural strata variable. For a fixed $K$, the ATCP is higher for maps with lower spatial resolution. For a fixed spatial resolution, the ATCP decreases with increasing $K$.

## References


[1] Daniel G Horvitz and Donovan J Thompson. A generalization of sampling without replacement from a finite universe. *Journal of the American statistical Association*, 47(260):663–685, 1952.

[2] Thomas Lumley and Others. Analysis of complex survey samples. *Journal of Statistical Software*, 9(1):1–19, 2004.

[3] Team, R Core. *R: A Language and Environment for Statistical Computing*. R Foundation for Statistical Computing, Vienna, Austria, 2018.

[4] Peter J Diggle and Emanuele Giorgi. *Model-based Geostatistics for Global Public Health: Methods and Applications, Section 5.3*. Chapman and Hall/CRC, 2019.

[5] C Edson Utazi, Julia Thorley, Victor A Alegana, Matthew J Ferrari, Saki Takahashi, C Jessica E Metcalf, Justin Lessler, and Andrew J Tatem. High resolution age-structured mapping of childhood vaccination coverage in low and middle income countries. *Vaccine*, 36(12):1583–1591, 2018.

[6] Håvard Rue, Sara Martino, and Nicolas Chopin. Approximate Bayesian inference for latent Gaussian models by using integrated nested Laplace approximations. *Journal of the Royal Statistical Society: Series B (Statistical Methodology)*, 71(2):319–392, 2009.

[7] National Population Commission - NPC and ICF. Nigeria Demographic and Health Survey 2018 - Final Report, 2019. Abuja, Nigeria: NPC and ICF. Available at `http://dhsprogram.com/pubs/pdf/FR359/FR359.pdf`.

[8] Daniel Simpson, Håvard Rue, Andrea Riebler, Thiago G Martins, Sigrunn H Sørbye, et al. Penalising model component complexity: A principled, practical approach to constructing priors. *Statistical Science*, 32(1):1–28, 2017.
